# Supplementary material for: Contact-Barrier Free, High Mobility, Dual-Gated Junctionless Transistor Using Tellurium Nanowire
Source: arXiv:2102.03507 source file (2021-02-06)
Supplement: Supplementary file 1 [file Supporting_Info.pdf]

# Supporting Information for: Contact-Barrier Free, High Mobility, Dual-Gated Junctionless Transistor Using Tellurium Nanowire

Pushkar Dasika,† Debadarshini Samantaray,‡ Krishna Murali,† Nithin Abraham,† Kenji Watanbe,¶ Takashi Taniguchi,§ N. Ravishankar,‡ and Kausik Majumdar*,†

†*Department of Electrical Communication Engineering, Indian Institute of Science, Bangalore 560012, India*

‡*Materials Research Center, Indian Institute of Science, Bangalore 560012, India*

¶*Research Center for Functional Materials, National Institute for Materials Science, 1-1 Namiki, Tsukuba 305-044, Japan*

§*International Center for Materials Nanoarchitectonics, National Institute for Materials Science, 1-1 Namiki, Tsukuba, 305-044 Japan*

E-mail: Kausikm@iisc.ac.in

## Supporting Figure 1: Cross section view of the nanowire transistor

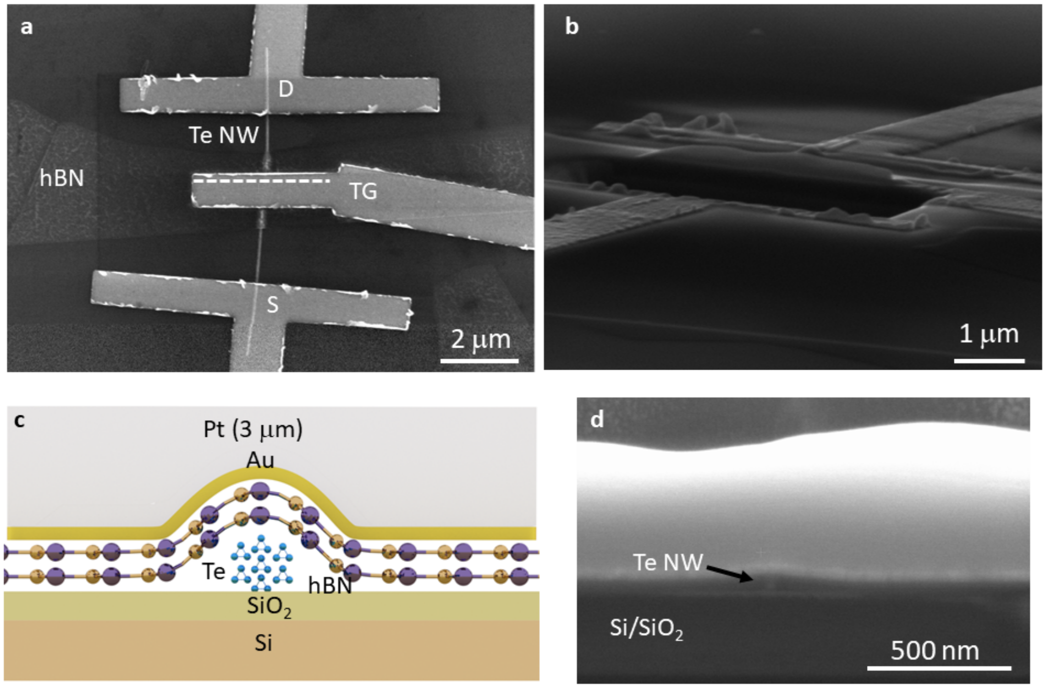


Figure 1: (a) Plan-view scanning electron micrograph for a nanowire FET. (b) Focussed ion beam cut along the dashed line in (a). (c-d) Schematic (in c) and scanning electron micrograph (in d) of the cross section of the device when cut along the dashed line in (a).

# Supporting Figure 2: Drift diffusion simulation of junctionless FET

To gain deeper understanding of operation of junctionless transistor, drift diffusion simulation have been performed assuming a charge sheet model and solving Shockley equations self consistently. Band gap of the material is assumed 0.6 eV, default doping is defined by $E_F - E_V = 0.2$ eV.

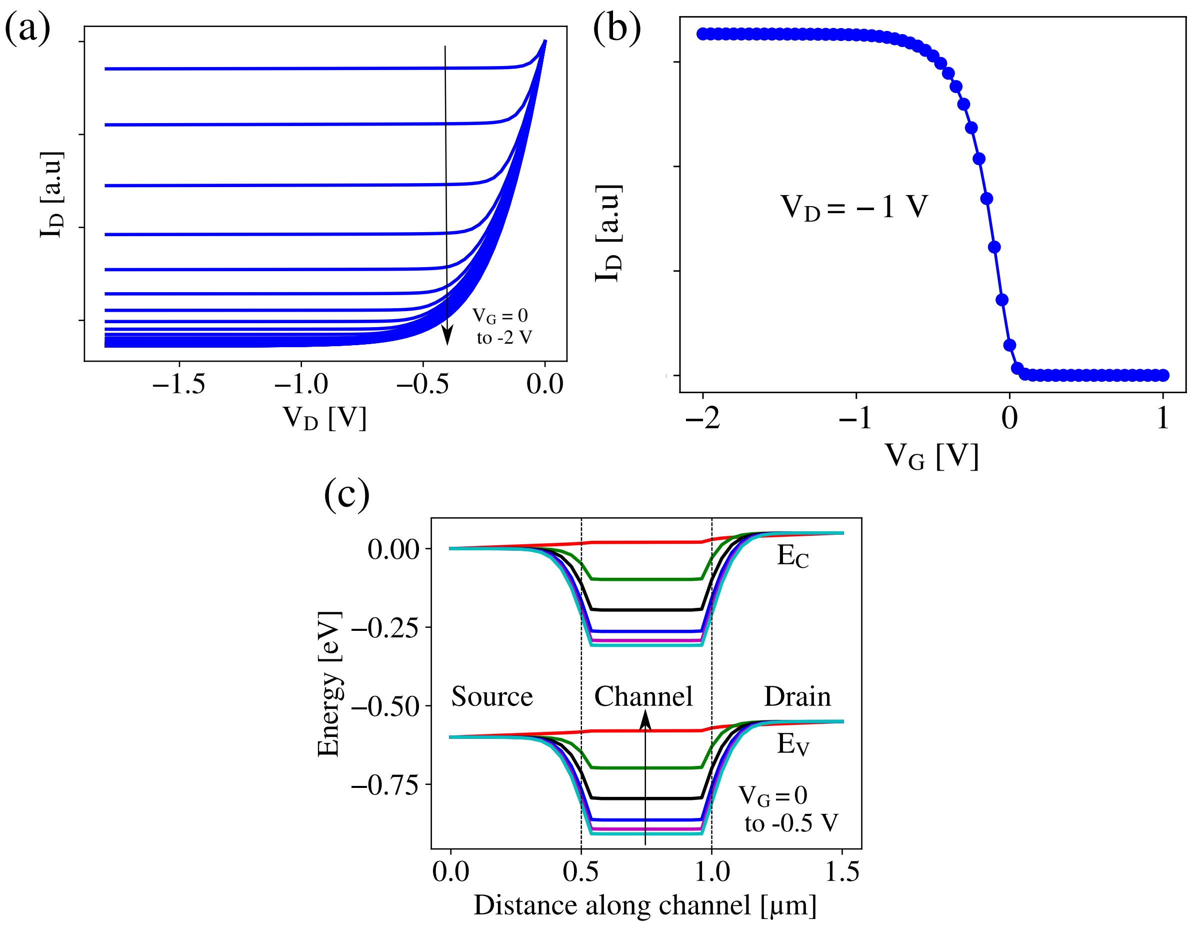


Figure 2: (a) Output and (b) transfer characteristics of the device showing the saturation of current at more negative top gate voltage. Although the characteristics follow square law near threshold, but start saturating at more negative gate bias. (c) Band profile of the device at various gate biases, keeping a small drain bias.
